# Supplementary material for: Per Garment Capture and Synthesis for Real-time Virtual Try-on
Source: arXiv:2109.04654 source file (2021-09-10)
Supplement: Supplementary file 1 [file supp-ablation.tex]

\section{Additional ablation studies}

\iccmt{Should we remove this one to the supplemental material?}
\paragraph{The usage of color-coded measurement garment}
We compared two measurement garment designs. 
One is regular t-shirt with a uniform color and the other is a t-shirt with the color-coded pattern.
The purpose is to evaluate the benefit of the usage of our custom-designed color-coded measurement garment.
In \figname~\ref{fig:ablation_use_measurement}, we can observe that the try-on results synthesized by the network trained with the uniform color measurement garment (top row in \figname~\ref{fig:ablation_use_measurement}) produce huge artifacts while the network trained with the color-coded measurement garment (bottom row in \figname~\ref{fig:ablation_use_measurement}) is better in depicting body shapes and preserving texture patterns on the target garments.

\begin{figure}[t!]
\centering
  \includegraphics[width=\linewidth]{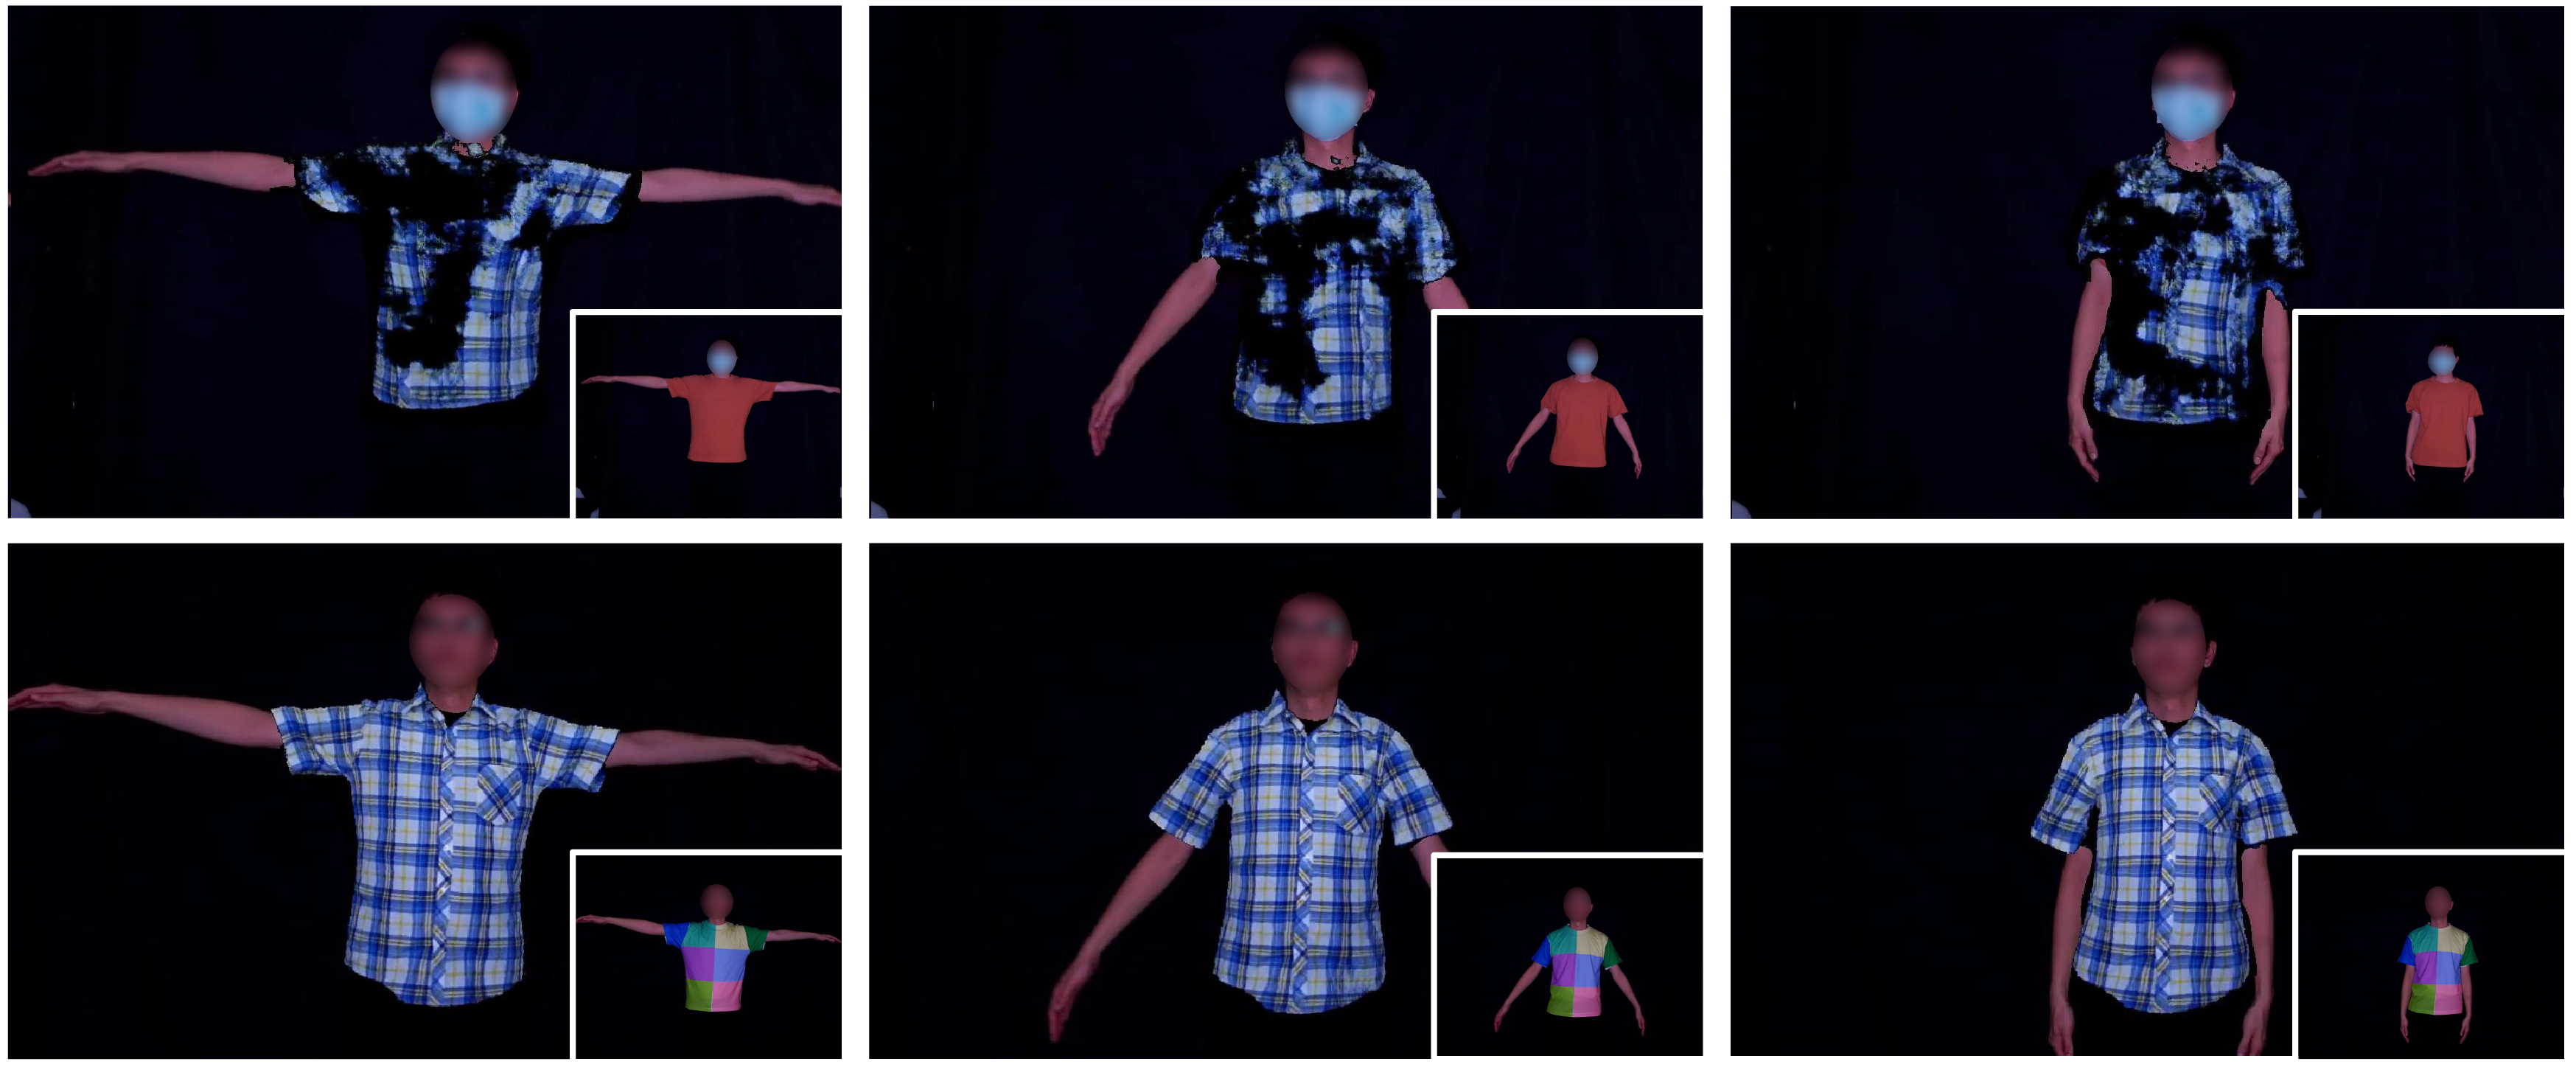}
  \caption{
  The usage of color-coded measurement garment.
  Top: the try-on results trained and tested with the T-shirt as the measurement garment.
  Bottom: the try-on results trained and tested with our custom-designed color-coded T-shirt as the measurement garment.
  We can see that the results synthesized with our custom-designed garment are better in depicting body shapes and texture pattern preservation.
  }
\label{fig:ablation_use_measurement}
\end{figure}

\paragraph{Garment deformation}\label{sec:deform_robust}
In our method, we did not explicitly model the underlying geometry in both capturing and synthesizing parts. 
However, as shown in \figname~\ref{fig:stretching}, our system can synthesize garment deformations during the try-on interactions.
The result is thanks to our per garment capturing and synthesizing workflow that extensively captures and models the target garment under various body poses and sizes.
For example, as the customer pulls down the garment, the garment shows reasonable stretching behavior. 
This would be difficult with an approach that synthesizes try-on images only from body joint locations.

\begin{figure}[t!]
\centering
  \includegraphics[width=\linewidth]{figures/deformation_fig.pdf}
  \caption{
  Garment deformation. Our system synthesizes natural and accurate garment deformation without explicitly model these deformations during capturing and synthesis. 
  (a) Input images where the user wears the measurement garment. (b) Virtual try-on results.
  Notice the grid pattern on the garment retains its structure and expand to response to stretch (the white dotted lines are used for referencing the garment's stretch).
  }
\label{fig:stretching}
\end{figure}
